# Supplementary material for: Is there an order-barrier $p\leq2$ for time integration in computational elasto-plasticity?
Source: arXiv:1512.06767 source file (2015-12-21)
Supplement: Supplementary file 1 [file appendix.tex]

\vfill
\newpage

\begin{center}
{APPENDIX A}
\end{center}

%-------------------------------------------------------------------------------------------------------------------------------
\section{Time discretization by implicit RK methods}
\label{sec:RKSolutionStepsForDAEs}
%==============================================================================================

To put things into perspective and for ready reference in the present paper, we briefly recall some basic 
equations for the solution of an initial value problem (IVP) by implicit RK (IRK) methods, cf. e.g. 
\cite{HaNoWaI, HaLuRo, HaWaII}. 
The IVP exhibits the format
\begin{equation}
\label{ivp}
\dot{\by} = \bbf(\by)\,,\qquad \by(t_0) = \by_0\,,\qquad t \in [t_0, T]
\end{equation}
which consists of an ordinary differential equation (ODE), \eqref{ivp}$_1$, along with initial conditions,
\eqref{ivp}$_2$. In \eqref{ivp} we drop for notational convenience the argument $\bE$ but keep in mind
that in computational inelasticity the IVP is embedded in a boundary value problem (BVP) which is solved
by finite elements resulting in displacements $\bu$ and total strains $\bE$. The total time interval
is decomposed into subintervals
$t_0 < t_1 < \ldots < t_n < \ldots < t_{n+1} < \ldots < t_N = T$, the \emph{time steps} with time step
size $\Delta t_{n}=t_{n+1}-t_{n}, 0 \leq n \leq N$. Assuming that the exact solution at $t_n$ is given
as $\by(t_n)$, the solution at $t_{n+1}$ is searched
\begin{equation}
\by(t_{n+1}) = \by(t_{n}) + \int_{t_n}^{t_{n+1}} \bbf(t, \by(t)) \mbox{d}t\,.
\end{equation}
For the numerical solution $\by_{n+1} \approx \by(t_{n+1})$ the integral is calculated by a quadrature rule 
consisting of $s$ stages
\begin{equation}
\label{integration-1}
\by_{n+1} = \by(t_n) + \Delta t_{n} \sum_{i=1}^s b_i \bbf(t_n + c_i \Delta t_{n}, \by(t_n + c_i \Delta t_{n}))
\end{equation}
with weighting factors $b_i, {i=1,...,s}$ and the coefficients $c_i, {i=1,...,s}$ where the latter 
define new time \emph{stages}
$t_i = t_n + c_i \Delta t_{n}$.
The unknowns $\by(t_n + c_i \Delta t_{n})$ are calculated by a second integration step in analogy to 
\eqref{integration-1} employing the same stages $c_i$ but along with the weighting factors $a_{ij}$ 
building the \textit{Runge-Kutta-Matrix} $A = (a_{ij})_{i,j=1,...,s}$, hence
\begin{equation}
\label{integration-2}
\bz(t_n + c_i \Delta t_{n}) \approx \bY_{ni} = \by(t_n) + \Delta t_{n} \sum_{j=1}^s a_{ij} \bbf(t_j,\bY_{nj}) \,, \qquad {i=1,...,s}\,.
\end{equation}
With
$\dot{\bY}_{nj}:=\bbf(t_{j}, \bY_{nj})$,
the \emph{stage derivatives},
we can rewrite \eqref{integration-2} as
\begin{equation}
\label{integration-3}
\bY_{ni} = \by(t_n) + \Delta t_{n} \sum_{j=1}^s a_{ij} \dot{\bY}_{nj} \,, \qquad {i=1,...,s}\,.
\end{equation}
% CK<
Hence, $\bY_{ni}$ and $\dot{\bY}_{ni}$ are two sets of unknowns which are related by \eqref{integration-3}.
After the calculation of the stage derivatives $\dot{\bY}_{ni}$ the update for $\by_{n+1}$ reads
\begin{equation}
\label{integration-4}
\by_{n+1} = \by_n + \Delta t_{n} \sum_{i=1}^s b_i \dot{\bY}_{ni}\,.
\end{equation}

RK methods exhibit \textit{stages} $c = (c_i)_{i=1,...,s}$, \textit{weighting vectors} $b=(b_i)_{i=1,...,s}$ 
and the \textit{Runge-Kutta-Matrix} $A = (a_{ij})_{i,j=1,...,s}$. A typical representation of RK methods is 
the so-called \textit{Butcher-array}, see Tab. \ref{tab:Butcher-Array-DAE}. 
For $s$-stage methods, $b,c\in\Real^s$ and $A\in\Real^{s\times s}$. Between the lines $a_{i.}$ of the RK 
matrix and the stages $c_i$ the following relationship holds $c_i = \Sum_{j=1}^s a_{ij}\,.$

\begin{table}[htbp]
\center
\begin{minipage}[b]{0.4\textwidth}

\center
\begin{tabular}{c|cccc}
   $c_1$   &  $a_{11}$  & $a_{12}$  &  $\ldots$  &  $a_{1s}$ \\
   $c_2$   &  $a_{21}$  & $a_{22}$  &  $\ldots$  &  $a_{2s}$ \\
 $\vdots$  &  $\vdots$  &           &  $\ddots$  &  $\vdots$ \\
   $c_s$   &  $a_{s1}$  & $a_{2s}$  &  $\ldots$  &  $a_{ss}$ \\
                                                     \hline
           &   $b_1$    &  $b_1$    &  \ldots    &  $b_s$    \\
\end{tabular}
\end{minipage}
\begin{minipage}[b]{0.4\textwidth}

\center
\begin{tabular}{c|cccc}
   $c_1$   &  $a_{11}$  &    $0$    &  $\ldots$  &     $0$   \\
   $c_2$   &  $a_{21}$  & $a_{22}$  &  $\ldots$  &     $0$   \\
 $\vdots$  &  $\vdots$  &           &  $\ddots$  &  $\vdots$ \\
   $c_s$   &  $a_{s1}$  & $a_{s2}$  &  $\ldots$  &  $a_{ss}$ \\
                                                     \hline
           &   $b_1$    &  $b_1$    &  \ldots    &  $b_s$    \\
\end{tabular}
\end{minipage}

\vspace*{2mm}

\begin{minipage}[b]{0.1\textwidth}
\center
\begin{tabular}{c|c}
     $1$ &   $1$  \\
\hline   &   $1$  \\
\end{tabular}
\end{minipage}
\begin{minipage}[b]{0.25\textwidth}
\center

\begin{tabular}{c|cc}
%               &                &                 \\
 $\dfrac{1}{3}$ & $\dfrac{5}{12}$ & $-\dfrac{1}{12}$ \\[2mm]
           $1$ & $\dfrac{3}{4}$  & $\dfrac{1}{4}$   \\[2mm]
                                             \hline \\[-6mm]
               & $\dfrac{3}{4}$  & $\dfrac{1}{4}$   \\

\end{tabular}
\end{minipage}
\begin{minipage}[b]{0.4\textwidth}
\center

\begin{tabular}{c|ccc}
 $\frac{4- \sqrt{6}}{10}$ & $\frac{88-7\sqrt{6}}{360}$ & $\frac{296-169\sqrt{6}}{1800}$ & $\frac{-2+3\sqrt{6}}{225}$ \\
 $\frac{4+\sqrt{6}}{10}$ & $\frac{296+169\sqrt{6}}{1800}$ & $\frac{88+7\sqrt{6}}{360}$ & $\frac{-2-3\sqrt{6}}{225}$ \\
 $1$ & $\frac{16-\sqrt{6}}{36}$ & $\frac{16+\sqrt{6}}{36}$ & $\frac{1}{9}$ \\
\hline  & $\frac{16-\sqrt{6}}{36}$ & $\frac{16+\sqrt{6}}{36}$ & $\frac{1}{9}$ \\
\end{tabular}
\end{minipage}
\caption{Butcher arrays (1st line, left) for implicit Runge-Kutta (IRK) methods, (1st line, right) for diagonally implicit RK (DIRK) methods 
and (2nd line, from left to right) Radau IIa-schemes for $s=1$, i.e. Backward-Euler, for $s=2$, and for $s=3$, respectively.
\label{tab:tab:Butcher-Array}}
\end{table}
 
The scheme is called \textit{algebraic stable}, \cite{HaNoWaI}, if the coefficients fulfil the two conditions
\begin{equation*}
\begin{array}{crcll}
(i)&b_i &\geq & 0, &i = 1,...,s\\
(ii)&M &:=&(b_i a_{ij} + b_j a_{ji}-b_i b_j)_{i,j=1,...,s}&\text{is positive semi-definite} \, .
\end{array}
\end{equation*}
 It can be shown that algebraic stable, implicit RK-methods are B-stable and for that reason also A-stable, 
 \cite{HaNoWaI}.
 Algebraic stable methods preserve the contractivity of plastic flow, \cite{BueSi}.
 This applies to RK-schemes of Radau IIa class, where the Butcher arrays for  $s\in\{1,2,3\}$ are summarized 
 in Tab.~\ref{tab:Butcher-Array-DAE}. 
 These three versions will be used in the present work.

The expected convergence order of the differential variables and the algebraic variable of the DAE system
%\eqref{Ind2-DAE-1}--\eqref{Ind2-DAE-3}
is listed in Tab. \ref{tab:ConvergenceOrder}, data taken from
Table VII.4.1 in \cite{HaNoWaI} and for the reduced order from \cite{BueSi}.
\begin{table}[htbp]

\center
\begin{tabular}{l c c }
\hline
variable type                               & convergence order &  reduced order   \\
\hline differential variable  $\by$      & $2s-1$            &       $2$        \\
       algebraic variable     $\gamma$      & $s$               &       $2$        \\
       \hline
\end{tabular}
\newline\newline
\caption{Global convergence order of the  $s$-stage ($s\geq2$) Radau IIa methods compared with order reduction for DAE systems. \label{tab:ConvergenceOrder}}
\end{table}

\begin{center}
{APPENDIX B}
\end{center}

%\textit{Acknowledgements}

\section*{General format of the equations within the partitioned ansatz}
\label{subsec:GeneralFormatPartitionedAnsatz}

As already explained, the key idea of the present contribution is to
replace linear interpolation for the construction of stage values for $\bu$ (or equally: $\bE$)
by quadratic interpolation, thus increasing the order of the corresponding approximation error to third order.
The ultimate aim of this procedure is to achieve consistency order 3 in time integration.
\\[2mm]
Equations \eqref{part-lin-vs-quad} are the general form of problem sets, where
the IVP for the ODE $\dot{\by} = \bbf(\bu,\by)$, see \eqref{ODE-GeneralFormat}, is solved by
RK methods within the partitioned ansatz.
\\[1mm]
\fbox{\parbox{14.2cm}{
%\hspace*{0mm}\parbox{14.5cm}{
\begin{equation}
\label{part-lin-vs-quad}
\begin{array}{lll}
%&\bu_{n+1} = \,\,\bP(\by_{n+1})&\\
&\left.\begin{array}{rcl}
                \bu_{n+1} &=& \,\,\bP(\by_{n+1}) \\[1mm]
                    \by_i &=& \by_n + \Delta t \Sum_{j=1}^s a_{ij} \bbf(\bu_j,\by_j) \\[1mm]
\mbox{lin.:} \quad \bu_i &=& \bu_n + c_i(\bu_{n+1}-\bu_n)                       \\
\mbox{quad.:} \quad \bu_i &=& \dfrac{c_i}{2}(c_i -1) \bu_{n-1} + (1-c_i^2) \bu_n + \dfrac{c_i}{2}(c_i+1) \bu_{n+1} \\[1mm]
                \by_{n+1} &=& \by_n + \Delta t \Sum_{i=1}^s b_i \bbf(\bu_i,\by_i)
\end{array}\right\}&i=1,...,s
\end{array}
\end{equation}
%}
}}
\\[4mm]
{\bf Remark:} \\
The compact expression \eqref{part-lin-vs-quad}$_1$ in terms of the operator $\bP$ shall be explained. For that aim we start out with the space-discrete format of the weak form of the balance of momentum. For notational convenience we choose here the geometrical linear case.

\begin{eqnarray}
0 &=&    \int_{\Omega^h} \bB^T \mathbb{C} \bB \, \mbox{d}\Omega \, \bu
       + \int_{\partial \Omega^h_{u}} \bB^T \, \mathbb{C} \, \bL  \, \bar{\bu} \, \mbox{d}\Omega    \nonumber \\ %\label{weak-1}
  & &  - \int_{\Omega^h} \bB^T \, \mathbb{C} \, \varepsilon^{p} \, \mbox{d}\Omega
       - \int_{\Omega^h} \bN^T \bbf \, \mbox{d}\Omega
       - \int_{\partial \Omega^h_{\sigma}} \bN^T \bar \Bsigma \, \mbox{d}\Omega_{\sigma}    \label{weak-1}\\
  &=& \bK \, \bu - {\bR}(\by) \label{weak-2}
\end{eqnarray}

where we use in \eqref{weak-2} the definition of the stiffness matrix $\bK$ and ${\bR}(\bz)$ for the remainder integrals
\begin{eqnarray}
          \bK &:=& \int_{\Omega^h} \bB^T \, \mathbb{C} \, \bB \, \mbox{d}\Omega        \label{stiffness-matrix}\\
        {\bR} &:=& - \int_{\Omega^h} \bB^T \, \mathbb{C} \, \varepsilon^{p} \, \mbox{d}\Omega
                      - \int_{\Omega^h} \bN^T \bbf \, \mbox{d}\Omega
                      - \int_{\partial \Omega^h_{\sigma}} \bN^T \bar \Bsigma \, \mbox{d}\Omega_{\sigma} \nonumber \\
                 &  & + \int_{\partial \Omega^h_{u}} \bB^T \, \mathbb{C} \, \bL  \, \bar{\bu} \, \mbox{d}\Omega \, .\label{matrix-R}
\end{eqnarray}
\\
Body forces in $\Omega$ are denoted by $\bbf$, external loads on boundary $\partial \Omega^h_{\sigma}$ by $\bar{\Bsigma}$, prescribed displacements
on boundary $\partial \Omega^h_{u}$ by $\bar u$. Finite element shape functions are denoted by $\bN$ and $\bL$ is a differential operator
calculating strains from displacements, $\bL:= \mbox{sym}(\triangledown) = 1/2(\triangledown + \triangledown^T)$, hence $\varepsilon= \bL\, \b u$.
% $\bL$ is a differential operator calculating strains from displacements, $\bL:= \mbox{sym}(\triangledown + \triangledown^T)$, hence $\varepsilon= \bL\, \bu$.
All integrals in \eqref{weak-1} are calculated by numerical quadrature, typically by the scheme of Gauss-Legendre. Here, we focus on the first integral in \eqref{matrix-R}
\begin{eqnarray}
\int_{\Omega^h} \bB^T \, \mathbb{C} \, \varepsilon^{p} \mbox{d}\Omega &\approx& \sum_{i=1}^{n_{gauss}} \alpha_i \, \bB^T(\xi_i) \, \mathbb{C} \, \varepsilon^{p}(\xi_i) \label{GaussLeg-1} %\\
%                                                             &=:& \bQ \, \varepsilon^{v} \label{GaussLeg-2}
\end{eqnarray}
with Gauss-points $\xi_i$ and Gauss-weights $\alpha_i$. Hence, \eqref{GaussLeg-1} and \eqref{weak-1} highlight the staggered/partitioned nature
in computational inelasticity where the weak form is solved for $\bu$ on a global level and the solution of the evolution equations for
$\varepsilon^p$ is solved on a local, Gauss-point level.

Discretisation in time for \eqref{weak-1} along with $\Delta t=t_{n+1}-t_n $ as time interval of interest yields the solution for the unknown displacements $\bu$ at $t_{n+1}$ according to \eqref{part-lin-vs-quad}$_1$ where $\bP:=\bK ^{-1} {\bR}$.
%\begin{equation}
%\bu_{n+1} = \bP(\bz_{n+1}):=\bK ^{-1} {\bR}(\bz_{n+1})
%\end{equation}
% which explains the format \eqref{part-lin-vs-quad}$_1$.
%-----------------------------------------------------------------------------------------------------------

\begin{center}
{APPENDIX C}
\end{center}

In this section we briefly summarise the result of \cite{EidelKuhn2010}, where it was shown
for the ODE case of viscoelasticity that it is a low-order approximation of the strain path
in time which is reason for order reduction.

More specifically, the interpolation techniques introduced in Sec. \ref{sec:Reasons4OrderReduction} and their effect on the
order of convergence of stress-update algorithms in computational elasto-plasticity are analysed.
For definiteness, we use a two-stage ($s=2$) Radau IIa method which exhibits
third order accuracy, ($p=3$).

The main result of this analysis in \cite{EidelKuhn2010} is summarized in the following Theorem 1.

%\begin{minipage}{14.0cm}

\fbox{\parbox{13.5cm}{
{\bf Theorem 1.}
For the partitioned system $\eqref{part-lin-vs-quad}_{1,2}$ the order of
consistency for $\bz$ is three, if quadratic interpolation for $\bu_i$
according to $\eqref{part-lin-vs-quad}_{4}$ is used and if the two-stage
Runge-Kutta method fulfills the following conditions:
\begin{equation}
\label{ConditionsFor3rdOrder}
\Sum_{i=1}^s b_i = 1,                 \hspace*{4mm}
\Sum_{i=1}^s b_i c_i = \frac{1}{2},   \hspace*{4mm}
\Sum_{i=1}^s b_i c_i^2 = \frac{1}{3}, \hspace*{4mm}
\Sum_{i=1}^s b_i\Sum_{j=1}^s a_{ij}c_j = \frac{1}{6}.
\end{equation}
Linear interpolation for $u_i$ according to $\eqref{part-lin-vs-quad}_{3}$
results in an order reduction of $\bz$ to order two.
%\end{minipage}
}}

\emph{Proof.} The proof is based on Taylor series expansion of the numerical
solution employing quadratic interpolation of $u$ as well as a Taylor expansion
of the exact solution. A comparison of coefficients in both solutions for the
requirement of third order convergence amounts to conditions \eqref{ConditionsFor3rdOrder}
for $a_{ij}$, $b_j$ and $c_i$ of the Runge-Kutta scheme which ensure the theoretical order
of consistency. These conditions are fulfilled by the applied Radau IIa scheme for $s=2$,
see Tab. \ref{tab:Butcher-Array-DAE}.

For convenience we slightly simplify the notation in the following. We write $u$ for $\bu$, $f$ for $\bbf$, $z$ for $\bz$ and use $h:=\Delta t$, $P$ for $\bf P$. Furthermore we use $P_z := \partial_z P$ for partial derivatives.

{\bf $\bullet$ \, Taylor series expansion of the numerical solution}
\\
Taylor expansion of the numerical solution $u_{n+1}$ at $z_n$ with
time increment $h:= \Delta t = t_{n+1} - t_n$ yields
\begin{eqnarray}
\label{ExpansionNumericalSolution}
u_{n+1} &=& P(z_{n+1}) = P(z_n + h\Sum_{i=1}^s b_i f(u_i,z_i))
%\nonumber
\\
\label{ExpansionNumericalSolution-1}
&=& P(z_n)
\\
&& + h\biggl( \Sum_{i=1}^s b_i f(u_i,z_i)\biggl) P_z(z_n)
\nonumber \\
&& + \frac{h^2}{2}\biggl( \Sum_{i=1}^s b_i f(u_i,z_i)\biggl)^2 P_{zz}(z_n)
\nonumber \\
&& + \frac{h^3}{6}\biggl( \Sum_{i=1}^s b_i f(u_i,z_i)\biggl)^3
P_{zzz}(z_n)  + \mathcal{O}(h^4) \nonumber.
\end{eqnarray}
An expansion of the terms $f(u_i,z_i)$ and $(u_n, z_n)$ is in order. The second term in \eqref{ExpansionNumericalSolution-1} is expanded to $\mathcal{O}(h^3)$, the third term in \eqref{ExpansionNumericalSolution-1} to $\mathcal{O}(h^2)$, the third term in  \eqref{ExpansionNumericalSolution-1} to order $\mathcal{O}(h)$. In the following we introduce Taylor-expansions for $f:=f(u_n, z_n)$ and drop for convenience the argument for function evaluations at $(u_n,z_n)$.
With $\du_i := u_i - u_n=\mathcal{O}(h)$ and $\dz_i := z_i - z_n=\mathcal{O}(h)$ it holds
\begin{eqnarray}
f(u_i,z_i) &=& f + \mathcal{O}(h), \\
f(u_i,z_i) &=& f + \du_i f_u + \dz_i f_z + \mathcal{O}(h^2),\label{e2}\\
f(u_i,z_i) &=& f + \du_i f_u + \dz_i f_z +
\dfrac{\du_i^2}{2}f_{uu} + \du_i\dz_i f_{uz} +
\dfrac{\dz_i^2}{2}f_{zz} + \mathcal{O}(h^3).\hspace{1cm} \label{e3}
\end{eqnarray}

{\bf $\bullet$ \, Taylor series expansion of the exact solution}
\\
For a comparison of coefficients the Taylor series expansion of the exact solution
must be determined
\begin{equation}
\label{ExpansionExactSolution}
u(t_n + h) = u + h \dot{u} + \frac{h^2}{2} \ddot{u} +
\frac{h^3}{6} \dddot{u} + \mathcal{O}(h^4) \, .
\end{equation}
Applying the chain rule and the product rule yields the time derivatives of $u$ in
\eqref{ExpansionExactSolution}
\begin{eqnarray}
\dot{u} &=& P_z f\\
\ddot{u} &=& P_{zz}f^2 + P_z^2 f f_u + P_z ff_z\\
\dddot{u} &=& P_{zzz}f^3 + 4P_{zz}P_z f^2 f_u + 3 P_{zz} f^2 f_z + 2 P_z^2 f f_u f_z + 2 P_z^2 f^2 f_{uz}
\nonumber \\
&& + P_z^3 f f_u^2 + P_z^3 f^2 f_{uu} + P_z f f_z^2 + P_z f^2 f_{zz}\, .
\end{eqnarray}

A comparison of coefficients in Taylor-expansions of \eqref{ExpansionNumericalSolution} and
\eqref{ExpansionExactSolution} will result in conditions for the Runge-Kutta time integrator
to achieve order two and order three, respectively.

{\bf $\bullet$ \, Conditions for order 2}
\\
A comparison of coefficients of $h$-terms and $h^2$-terms yields the same conditions for
consistency order two as in \cite{Buettner-Disse}, since $\tilde{c}_i$ (stemming from
quadratic interpolation) merely appears in $h^3$-terms.
Hence, the conditions stemming from a comparison of $h$- and $h^2$-terms read

\fbox{\parbox{13.5cm}{
%   {\bf General:} $J(y) = J[y(x)]$ \quad Function of a function = functional
\begin{equation}
%\fbox{
%\hspace*{1cm}
\Sum_{i=1}^s b_i = 1\hspace{1cm}\text{and}\hspace{1cm}
\Sum_{i=1}^s b_i c_i = \frac{1}{2}\, .
\label{Bed2}
%\hspace*{1cm}
%}
\end{equation}
   }}

{\bf $\bullet$ \, Conditions for order 3}
\\

Summarizing, two additional conditions for order three are imposed to the RK method:

\fbox{\parbox{13.5cm}{
\begin{equation}
\Sum_{i=1}^s b_i c_i^2 =
\frac{1}{3}\hspace{1cm}\text{and}\hspace{1cm} \Sum_{i=1}^s b_i
\Sum_{j=1}^s a_{ij}c_j = \frac{1}{6} \, , \label{ZusBed3}
\end{equation}
}}

which are both fulfilled by the coefficients of Radau IIA-schemes with $s\geq 2$,
see the Butcher array in the right of Table \ref{tab:Butcher-Array-DAE}.

It is worth to note that the proof is based on problems that are described by an ODE.
For the broad class of computational inelasticity this applies to
constitutive equations either of (rate dependent) viscoelasticity or to models
of elasto-plasticity \emph{without} yield surfaces as an algebraic constraint like
the model of Chan-Bodmer-Lindholm etc. For models of (rate-independent) elasto-plasticity
entailing a yield surface and thus forming a DAE this proof does not apply.
